# Supplementary material for: Elastic constants of graphene: Comparison of empirical potentials and DFT calculations
Source: arXiv:1902.04855 ancillary file (2019-02-13)
Supplement: Supplementary file 1 [file SI.pdf]

# Supplementary Information to "Elastic constants of graphene: Comparison of empirical potentials and DFT calculations"

Irina V. Lebedeva,[1,*] Alexander S. Minkin,[2,†] Andrey M. Popov,[3,‡] and Andrey A. Knizhnik[4,§]

[1]*Nano-Bio Spectroscopy Group and ETSF, Universidad del País Vasco, CFM CSIC-UPV/EHU, Avenida de Tolosa 72, San Sebastian 20018, Spain*

[2]*National Research Centre "Kurchatov Institute", Kurchatov Square 1, Moscow 123182, Russia*

[3]*Institute for Spectroscopy of Russian Academy of Sciences, Fizicheskaya Street 5, Troitsk, Moscow 108840, Russia*

[4]*Kintech Lab Ltd., 3rd Khoroshevskaya Street 12, Moscow 123298, Russia*

## COMPARISON OF COMPUTATIONAL EFFICIENCY OF INTERATOMIC POTENTIALS

To illustrate the computational effort associated with the use of the Tersoff [1], REBO-2000 [2], AIREBO [2], PPBE-G [3], LCBOP [4], ReaxFF-CHO [5] and ReaxFF-C2013 [6] potentials, we performed molecular dynamics simulations using the LAMMPS code [7]. The (2000,0) CNT was considered. The simulation cell included 6 elementary unit cells along the nanotube axis. The calculations were carried out in the microcanonical ensemble using the velocity Verlet algorithm [8, 9]. 100 molecular dynamics steps of 0.05 fs duration were performed.

The serial version of LAMMPS from the 16th of March of 2018 was used. The test calculations for the comparison of CPU times were carried out using a personal computer with the processor Intel(R) Core(TM) i7-3770 CPU @ 3.40GHz and memory RAM of 8Gb. Distinct computational performance is possible for different potentials using other computer architectures (MPI, OpenMP, CUDA, OpenCL, etc.) and hardware [10] and the corresponding detailed analysis is beyond the scope of the present paper.

The CPU time computed from the molecular dynamics tests (Table I) is the smallest for PPBE-G [3]. Indeed this potential has the simplest form among the potentials considered. As the complexity of the expression for the potential energy grows and long-range interactions are included, the calculations become heavier. The computational time thus increases in the row: PPBE-G $<$ Tersoff $<$ LCBOP $\approx$ REBO-2000 $<$ AIREBO $<$ ReaxFF-C2013 $\lesssim$ ReaxFF-CHO.

TABLE I. CPU times corresponding to 100 molecular dynamics steps of 0.05 fs duration performed using a personal computer with the processor Intel(R) Core(TM) i7-3770 CPU @ 3.40GHz and memory RAM of 8Gb.

| Method | CPU time (s) |
|---|---|
| Tersoff [1] | 11.621 |
| AIREBO [2] | 49.118 |
| REBO-2000 [2] | 19.029 |
| LCBOP [4] | 18.233 |
| PPBE-G [3] | 4.370 |
| ReaxFF-CHO [5] | 203.79 |
| ReaxFF-C2013 [6] | 156.85 |

## DATA AVAILABILITY

The scripts and input files required to reproduce these findings are available to download from https://data.mendeley.com/datasets/nnd9d4y2mb/2.

## REFERENCES

* liv_ira@hotmail.com
† amink@mail.ru
‡ popov-isan@mail.ru
§ kniznik@kintechlab.com

[1] J. Tersoff, "Empirical interatomic potential for carbon, with applications to amorphous carbon," Phys. Rev. Lett. **61**, 2879–2882 (1988).

[2] S. J. Stuart, A. B. Tutein, and J. A. Harrison, "A reactive potential for hydrocarbons with intermolecular interactions," J. Chem. Phys. **112**, 6472–6486 (2000).

[3] D. Wei, Y. Song, and F. Wang, "A simple molecular mechanics potential for $\mu$m scale graphene simulations from the adaptive force matching method," J. Chem. Phys. **134**, 184704 (2011).

[4] J. H. Los and A. Fasolino, "Intrinsic long-range bond-order potential for carbon: Performance in Monte Carlo simulations of graphitization," Phys. Rev. B **68**, 024107 (2003).

[5] K. Chenoweth, A. C. T. van Duin, and W. A. Goddard, "ReaxFF reactive force field for molecular dynamics simulations of hydrocarbon oxidation," J. Phys. Chem. A **112**, 1040–1053 (2008).

[6] S. G. Srinivasan, A. C. T. van Duin, and P. Ganesh, "Development of a ReaxFF potential for carbon condensed phases and its application to the thermal fragmentation of a large fullerene," J. Phys. Chem. A **119**, 571–580

(2015).

[7] S. Plimpton, "Fast parallel algorithms for short-range molecular dynamics," J. Comp. Phys. **117**, 1–19 (1995).

[8] M. P. Allen and D. J. Tildesley, *Computer Simulation of Liquids* (Computer Simulation of Liquids, 1987).

[9] W. C. Swope, H. C. Andersen, P. H. Berens, and K. R. Wilson, "A computer simulation method for the calculation of equilibrium constants for the formation of physical clusters of molecules: Application to small water clusters," J. Chem. Phys. **76**, 637–649 (1982).

[10] A. S. Minkin, A. A. Knizhnik, and B. V. Potapkin, "GPU implementations of some many-body potentials for molecular dynamics simulations," Advances in Engineering Software **111**, 43–51 (2017).
